# Supplementary material for: Adaptive Fully Dynamic $k$-Center Clustering with (Near-)Optimal Worst-Case Guarantees
Source: arXiv:2604.01726 source file (2026-04-02)
Supplement: Supplementary file 1 [file appendix.tex]

\section{Extending~\cref{thm:bicr_alg_merged} to $(k, z)$-Clustering}
\label{appendix:k_z_clustering}
